# Supplementary material for: ChannelExplorer: Exploring Class Separability Through Activation Channel Visualization
Source: arXiv:2505.04647 source file (2025-05-06)
Supplement: Supplementary file 1 [file 99-supplementary.tex]

\clearpage
\setcounter{page}{1}
\onecolumn
 % Prefix sections with "S"
\setcounter{section}{0} % Reset section counter
% Centered title for Supplementary Materials
\begin{center}
    {\LARGE\textbf{Supplementary Materials}}
\end{center}

\section{ImageNet Dataset Findings}

We used \toolname{} to reduce inter-class and intra-class confusion for the InceptionV3 model pre-trained on the ImageNet dataset. Exploring using \toolname{}, we found different ways to create a class hierarchy to reduce class confusion. ImageNet class labels were created using Wordnet synset hierarchy. Wordnet has 60942 nodes in its synset word hierarchy, from which ImageNet used 2155 nodes. It is reasonable to find similarities between ImageNet classes that are under the same parent node in Wordnet. The examples shown here are different hierarchies than wordnet that were found while exploring \toolname{}.

% https://observablehq.com/@mbostock/imagenet-hierarchy

\subsection{Super-classification Examples}

This subsection provides examples of super-classification using \jaccardcolor{Jaccard Similarity View} in \cref{fig:suppl-jaccard1} and \cref{fig:suppl-jaccard2}. The darker groups between the two classes in each \jaccardcolor{Jaccard Similarity View} mean they have strong activation similarities.

\begin{figure}[ht]
    \centering
    % First subfigure
    \begin{subfigure}[b]{0.45\textwidth}
        \centering
        \includegraphics[width=\textwidth]{figs/supplementary/superclassification-1.png}
        \caption{Digital Clock (3rd class), Digital Watch (4th class) and Stopwatch (5th class) form a super-class. Wall clocks (6th class) and Analog clocks (2nd class) form a super-class.}
        \label{fig:suppl-jaccard1}
    \end{subfigure}
    \hfill
    % Second subfigure
    \begin{subfigure}[b]{0.45\textwidth}
        \centering
        \includegraphics[width=\textwidth]{figs/supplementary/superclassification-2.png}
        \caption{Pay-phone (5th class) and Dial telephone (2nd class) form a super-class.}
        \label{fig:suppl-jaccard2}
    \end{subfigure}
    \caption{Examples of super-classification with \jaccardcolor{Jaccard Similarity View}.}
    \label{fig:main}
\end{figure}

\subsection{Sub-classification Examples}
\cref{fig:suppl-scatterplot} shows examples of sub-classifications that were done using the \scattercolor{Scatterplot View}.

\subsection{Retraining InceptionV3 with new Sub-classes}
\label{supsec:retraining}
After identifying subclasses, the retraining process was completely manual. We removed the last fully connected layer and replaced it with a new fully connected layer of 1002 neuron units. The weights of this layer are randomly initialized (Xavier initialization method is used). The training is done with 50 epochs over the modified training data with new sub-classes. To create the new subclasses, we first used the previous clusters to divide the class. Then, we manually went through each sub-class to evaluate whether the semantics of these sub-classes made sense (i.e., there are really Bisons in cold weather in the sub-class \textit{cold-bison}). We compared the per-class accuracy for the common subset of classes and the macro-F1 score for all classes.

\begin{figure*}[ht!]
\centering

% Row 1
\begin{subfigure}[b]{0.295\linewidth}
\includegraphics[width=\linewidth]{figs/supplementary/subclassification-2.png}
\caption{Labrador Retriever: White dog vs. Black dog}
\end{subfigure}
\hfill
\begin{subfigure}[b]{0.295\linewidth}
\includegraphics[width=\linewidth]{figs/supplementary/subclassification-3.png}
\caption{Basenji: Western Pet Leanage vs. African Leanage}
\end{subfigure}
\hfill
\begin{subfigure}[b]{0.295\linewidth}
\includegraphics[width=\linewidth]{figs/supplementary/subclassification-4.png}
\caption{Red Wolf: Summer vs. Winter Wolf}
\end{subfigure}

% Row 2
\begin{subfigure}[b]{0.295\linewidth}
\includegraphics[width=\linewidth]{figs/supplementary/subclassification-5.png}
\caption{Mongoose: Desert vs. City Mongoose}
\end{subfigure}
\hfill
\begin{subfigure}[b]{0.295\linewidth}
\includegraphics[width=\linewidth]{figs/supplementary/subclassification-6.png}
\caption{Stove: Chimney vs. Stove}
\end{subfigure}
\hfill
\begin{subfigure}[b]{0.295\linewidth}
\includegraphics[width=\linewidth]{figs/supplementary/subclassification-7.png}
\caption{Spider Web: Empty vs. Occupied Spider Web}
\end{subfigure}

% Row 3
\begin{subfigure}[b]{0.295\linewidth}
\includegraphics[width=\linewidth]{figs/supplementary/subclassification-8.png}
\caption{Refrigerator: Open vs. Closed}
\end{subfigure}
\hfill
\begin{subfigure}[b]{0.295\linewidth}
\includegraphics[width=\linewidth]{figs/supplementary/subclassification-9.png}
\caption{Pickelhaube: Worn vs. Unworn}
\end{subfigure}
\hfill
\begin{subfigure}[b]{0.295\linewidth}
\includegraphics[width=\linewidth]{figs/supplementary/subclassification-10.png}
\caption{Harmonica: Still vs. Playing}
\end{subfigure}

% Row 4
\begin{subfigure}[b]{0.295\linewidth}
\includegraphics[width=\linewidth]{figs/supplementary/subclassification-11.png}
\caption{Dishwasher: Closed vs. Open}
\end{subfigure}
\hfill
\begin{subfigure}[b]{0.295\linewidth}
\includegraphics[width=\linewidth]{figs/supplementary/subclassification-12.png}
\caption{Diaper: Worn vs Unworn}
\end{subfigure}
\hfill
\begin{subfigure}[b]{0.295\linewidth}
\includegraphics[width=\linewidth]{figs/supplementary/subclassification-1.png}
\caption{Oxen: Muskox vs. Bull}
\end{subfigure}
\caption{Activation Distance \scattercolor{Scatterplot View} of InceptionV3 model with different classes of ImageNet dataset. Each scatterplot shows visual clusters, and the columns on corresponding sides show four examples of each cluster. Some cluster separations are for obvious feature distinctions, and some separations are unintuitive.}
\label{fig:suppl-scatterplot}
\end{figure*}

\section{Model \& Dataset Exploration}
We tested \toolname{} on many Image-based models including AlexNet, VGGN16, VGG19, GoogLeNet, ResNet, DenseNet, EfficientNet, ConvNeXt, CoAtNet, DCGAN, StyleGAN2 and BigGAN. 
For consistency, we used the Imagenet dataset and the InceptionV3 CNN model throughout the paper. 
InceptionV3 with some convolution and concatenation layers are shown in \cref{fig:suppl-inceptionv3-imagenet-activation-argmax}. 
VGG16 model with a smaller imagenet dataset is shown in figure \cref{fig:suppl-vgg16-imagenette}. 

\begin{figure*}[ht]
    \centering
    \includegraphics[width=\linewidth]{figs/supplementary/inception-only-merge-activation-argmax.png}
    \caption{InceptionV3 model with only the Concatenation layers as they represent previous CNN layers' submodule. ImageNet is used as the dataset. Layer conv2d shows raw activation channels for all inputs, layer mixed8 shows \jaccardcolor{Jaccard Similarity View} where we see three classes of sharks form a super-class. Layer mixed9 and mixed10 show the \scattercolor{Scatterplot View} and \heatmapcolor{Heatmap View}. Finally, the prediction layer shows the model prediction for each input using the Argmax section. }
    \label{fig:suppl-inceptionv3-imagenet-activation-argmax}
\end{figure*}

\begin{figure*}[ht]
    \centering
    \includegraphics[width=\linewidth]{figs/supplementary/vgg15-imagenette.png}
    \caption{VGG16 model is shown with \textit{tench} and \textit{parachute} classes loaded from a customized version of the ImageNet dataset with 10 classes. The \scattercolor{Scatterplot View} are shown in all the layers. It shows that the model is successful in separating the images by their classes from the starting layers, although some images of the parachutes are misclassified as tech.  }
    \label{fig:suppl-vgg16-imagenette}
\end{figure*}

% TODO
% 1. Add SRGAN jaccard similarity
% 2. Add the channel vs mAP table/chart
\section{Inter-class confusions in SRGAN}
\cref{fig:srgan-jaccard} shows activation similarity of the last convolutional block of the SRResNet model. The similarity between \textit{orangutan} \& \textit{Persian cat} and \textit{coral reef} \& \textit{cliff} is visible in the similarity matrix.

\begin{figure}[ht]
    \centering
    \includegraphics[width=0.4\linewidth]{figs/supplementary/srgan-jaccard.png}
    \caption{\jaccardcolor{Jaccard Similarity View} of 5 classes of SRGAN. The similarity between \textit{orangutan} \& \textit{Persian cat} and \textit{coral reef} \& \textit{cliff} is visible in the similarity matrix.}
    \label{fig:srgan-jaccard}
\end{figure}

\section{Channel Pruning of CNN}
\label{supsec:pruning}

We removed activation channels from the bottom of the \heatmapcolor{Heatmap View} and recorded the performance difference of the whole model on the ImageNet evaluation dataset. We notice no change in performance even after 74\% of the activation channels. Model performance and speed for removing different numbers of activation channels in mixed10 layer is shown in \cref{tab:cnn_channels}.

\begin{table}[ht]
\centering

\setlength{\tabcolsep}{10pt}
\begin{tabular}{|c|c|c|c|}
\hline
\textbf{CNN Channels Left} & \textbf{Total Parameters} & \textbf{mAP} & \textbf{FPS} \\ \hline
100\%             & 3,333,120        & 0.500 & 16.62 \\ \hline
96\%              & 3,238,764        & 0.502 & 16.39 \\ \hline
83\%              & 2,945,836        & 0.505 & 16.19 \\ \hline
60\%              & 2,410,124        & 0.501 & 16.17 \\ \hline
26\%              & 1,596,297        & 0.502 & 16.32 \\ \hline
24\%              & 1,569,638        & 0.500 & 16.04 \\ \hline
23\%              & 1,536,326        & 0.497 & 14.48 \\ \hline
19\%              & 1,453,190        & 0.333 & 7.67  \\ \hline
17\%              & 1,396,832        & 0.025 & 7.15  \\ \hline
10\%              & 1,234,942        & 0.001 & 7.45  \\ \hline
\end{tabular}
\caption{Performance metrics based on the number of channels taken from the mixed10 layer of InceptionV3 model. }
\label{tab:cnn_channels}
\end{table}

We compared our interpretable manual pruning with two variants of VGG16 pruned using established techniques: (1) unstructured magnitude-based weight pruning, and (2) structured filter pruning based on norm values, both reducing 40\% of weights in the layers. We found that both pruned models have accuracy comparable to our manually pruned model. However, our method offers the additional advantage of selectively fine-tuning the accuracy trade-offs between classes.

\section{Stable Diffusion}
The input texts of the stable diffusion model that were used to produce the results of \cref{sec:use-case-stable-diffusion} are presented in \cref{tab:stable-diffusion-inputs}. All the 100 input texts and their corresponding outputs are presented in \cref{fig:sd-input-output}.

\newcolumntype{P}[1]{>{\raggedright\arraybackslash}p{#1}}

\begin{table}[]
    \centering
    \begin{tabular}{|P{0.45\linewidth}|P{0.45\linewidth}|}
\hline
\textcolor[HTML]{d5d540}{1. Misty river winding through rolling green hills at sunrise.} \newline
\textcolor[HTML]{d5d540}{2. Peaceful village surrounded by rice paddies and misty hills.} \newline
\textcolor[HTML]{d5d540}{3. Morning mist rising from a forest river with birds singing.} &
\textcolor[HTML]{69f741}{1. Peaceful village market with handcrafted goods and lively chatter.} \newline
\textcolor[HTML]{69f741}{2. Bustling cafe terrace in Paris with Eiffel Tower in view.} \newline
\textcolor[HTML]{69f741}{3. Bustling market square with jugglers, musicians, and merchants shouting wares.} \\
\hline
\textcolor[HTML]{ee4a7e}{1. Scenic mountain road winding through lush valleys and cliffs.} \newline
\textcolor[HTML]{ee4a7e}{2. Sunlit canyon with soaring cliffs and a winding river below.} \newline
\textcolor[HTML]{ee4a7e}{3. Windy cliffside path overlooking an endless expanse of the ocean.} &
\textcolor[HTML]{8f45f9}{1. Remote island with tropical plants, sandy shores, and crystal-clear water.} \newline
\textcolor[HTML]{8f45f9}{2. Sunny vineyard with rows of grapevines stretching into the distance.} \newline
\textcolor[HTML]{8f45f9}{3. Rainforest scene with parrots flying and waterfalls in the distance.} \\
\hline
    \end{tabular}
    \caption{The input prompts of each generated images of \cref{fig:scene-stable-diffusion}. }
    \label{tab:stable-diffusion-inputs}
\end{table}

\begin{figure}[ht]
    \centering
    \includegraphics[width=\linewidth]{figs/supplementary/gan-input-outputs.png}
    \caption{Inputs and corresponding outputs of the experiment of \cref{sec:use-case-stable-diffusion}. }
    \label{fig:sd-input-output}
\end{figure}

\section{Interface Details}

\para{Tutorial for new users.}
When the interface is launched for the first time, a tutorial will walk the user through each sections in the system. \Cref{fig:tutorial-combined}(A) shows a tutorial description of a layer node in the interface.

\para{Comprehensive Image View in \scattercolor{Scatterplot View}}
Hovering over the scatterplot will show a button at the top-left corner, which will change each point in the scatterplot with the corresponding image. \Cref{fig:tutorial-combined} (B) demonstrates this feature. The legends are also updated accordingly. 

\para{Horizontal Bar-chart for class overlap detection.}
Besides the scatterplot view, we also provide a horizontal barchart, showing the overlaps of classes in each cluster. In the barchart, each row represents how many images from each class are in that cluster. \Cref{fig:tutorial-combined}(B) shows that there are overlaps in the fourth cluster, highlighting confusion. Hovering over each bar will show the number of inputs in that cluster from the corresponding class. 

\begin{figure}[ht]
    \centering
    \begin{minipage}[b]{0.48\linewidth}
        \centering
        \includegraphics[width=\linewidth]{figs/supplementary/tutorial.png}
        \caption*{(A)}
    \end{minipage}
    \hfill
    \begin{minipage}[b]{0.48\linewidth}
        \centering
        \includegraphics[width=\linewidth]{figs/supplementary/scatterplot-image.png}
        \caption*{(B)}
    \end{minipage}
    \caption{(A) A tutorial describing a part of the interface. (B) A \scattercolor{Scatterplot View} showing all images at once.}
    \label{fig:tutorial-combined}
\end{figure}

\para{Selection across linked views. }
The selection of input is globally linked across all views in the interface. Selecting an image in the \datasetcolor{Dataset View} will also highlight the same example in all open views throughout all layers in the neural network overview and vice versa. 

\para{Remove visualization of models and datasets.}
One of the primary reasons for maintaining decoupled deployable backend and frontend design is to enable removal visualization for large neural networks. Often, the large models are run on machines with no display server attached to them. Rendering an integrated visualization system will not be possible for live visualization in these machines. We take the web-based decoupled frontend and backend visualization approach, where the backend can run beside the model in the same machine, while the frontend can be run on any remote machine, connected to the backend. This enables both remote visualization and simultaneous online collaboration among teams.
